# Supplementary material for: Fast and Provable Tensor Robust Principal Component Analysis via Scaled Gradient Descent
Source: arXiv:2206.09109 source file (2023-02-22)
Supplement: Supplementary file 1 [file appendix.tex]

%\input{appendix-aux.tex}

%\input{appendix-alg.tex}
